# Supplementary material for: EM-Assist: Safe Automated ExtractMethod Refactoring with LLMs
Source: arXiv:2405.20551 source file (2024-05-31)
Supplement: Supplementary file 1 [file appendix.tex]

\newpage
\appendix

\section{Artifacts Appendix}

Below we provide a walkthrough of the actual tool demonstration. To capture the attention of the participants, we envision a healthy balance of interactive live demos and the supporting slides: 
\begin{itemize}
    \item quickly describe problems caused by long methods 
    \item live demo of the standard Extract Method refactoring in IntelliJ IDEA
    \item overview of the research on ExtractMethod suggestion, and its shortcomings
    \item the key idea: the synergy between LLMs and IDEs, and the pros and cons of using LLMs for suggesting and executing refactorings.
    \item live demo of performing an ExtractMethod on a real-world Java long method, explaining the workflow from Figure~\ref{fig:example2}.
    \item live demo of performing an ExtractMethod on a real-world Kotlin long method, following the workflow from Figure~\ref{fig:example2}.
    \item summary of the Effectiveness evaluation results (\cref{sec:effectiveness})
    \item summary of the Usability evaluation results  (\cref{sec:user_eva})
    \item concluding slide with QR codes to download our plugin from the JetBrains Marketplace, the GitHub page, acknowledgements.
\end{itemize}

A link to a screencast of the envisioned workflow described above:
\url{https://www.youtube.com/watch?v=3E6KsHAg3js}

Our tool is freely available to install from the JetBrains Marketplace, the official repo of IntelliJ plugins:
\url{https://plugins.jetbrains.com/plugin/23403-llm-powered-extract-method}

Our tool is released under open-source license on GitHub. We include the source code, the evaluation data, sample LLM prompts and results, readme, etc:
\url{https://github.com/llm-refactoring/llm-refactoring-plugin}

\balance
